# Supplementary material for: Thermodynamic size control in curvature-frustrated tubules: Self-limitation with open boundaries
Source: arXiv:2109.01174 ancillary file (2021-09-02)
Supplement: Supplementary file 1 [file SI.pdf]

# Thermodynamic size control in curvature-frustrated tubules: Self-limitation with open boundaries Supplementary information

Botond Tyukodi,[1] Farzaneh Mohajerani,[1] Douglas M. Hall,[2] Gregory M. Grason,[2] and Michael F. Hagan[1]

[1] *Brandeis University, Waltham, USA*

[2] *UMass Amherst, Amherst, USA*

(Dated: September 2, 2021)

# I. THE MODEL

In this section we provide additional details about the model and Monte Carlo simulation that we used to generate the results in the main text. The model and algorithm are similar to the one used to describe microcompartment assembly in ref. [1] by Rotskoff and Geissler (which we refer to as the RG model henceforth). In particular, we consider flexible triangular subunits which can bind to each other along edges with a set of preferred dihedral angles that set the preferred curvatures of the assembling sheet. Monte Carlo simulations are performed in the grand canonical ensemble at fixed $\mu VT$, with $\mu$ the chemical potential of subunits in the bath. Each Monte Carlo simulation involves a single cluster undergoing assembly and disassembly, with subunits taken from or returned to the bath respectively, as well as structural relaxation moves. We describe specific differences with respect to the RG model below.

### 1. *Energies*

In the trumpet model, each three edges of the triangular subunits are of different types, $t(p) = 1, 2, 3$, for edge index $p$ and each edge can only bind to an edge of the same type on a neighboring subunit.

The total energy of the system is given by

$$E = \sum_{p}^{3n_{\rm s}} E^{p}_{\rm stretch} + \frac{1}{2}\sum_{\langle pq\rangle} (E^{pq}_{\rm bend} + E^{pq}_{\rm bind}) \tag{1}$$

where the first sum goes over all edges, with $n_{\rm s}$ the number of subunits in the cluster. The second sum only goes over bound edges (i.e. non-boundary, adjacent edges, so there are $2n_{\rm b}$ terms in the sum, with $n_{\rm b}$ as the number of bonds). The $1/2$ factor corrects for double counting.

The stretching energy is defined as:

$$E^{p}_{\rm stretch} = \epsilon_{\rm s}\frac{(l^p - l_0)^2}{2} \tag{2}$$

where $\epsilon_{\rm s}$ is the stretching modulus, $l^p$ is the instantaneous length, and $l_0$ is the stress-free (rest) length of an edge. For the trumpet model we set the stretching modulus and rest length equal for all edges.

The bending energy is quadratic in deviations from the preferred dihedral angle:

$$E^{pq}_{\rm bend} = \kappa_{\rm b}\frac{\left(\theta^{pq} - \theta_0^{t(p)t(q)}\right)^2}{2} \tag{3}$$

with $p$ and $q$ adjacent edges and $t(p), t(q)$ the edge types. $\kappa_{\rm b}$ is the bending modulus and is set equal for all edge types. $\theta_0^{t(p)t(q)}$ is the preferred dihedral angle between edges with types $t(p)$ and $t(q)$. Since only edges of the same types are allowed to bind to each other, $t(p) = t(q) \equiv t$ for all adjacent edge pairs $pq$, and $\theta_0^{t(p)t(q)} \equiv \theta_0^t$. Two of the types are set to have the same, positive preferred dihedral $\theta_0^1 = \theta_0^2 \equiv \theta_0^{\perp}$ and the third one is set to have a different, negative preferred dihedral $\theta_0^3 \equiv \theta_0^{\parallel}$.

The binding energy between two edges $p$ and $q$ (with the same type $t(p) = t(q) = t$) is given by

$$E^{t}_{\rm bind} = \epsilon^{t}_{\rm b} \tag{4}$$

Similar to the preferred dihedrals, the two binding energies corresponding to the $\theta_0^{\perp}$ edges are set equal to $\epsilon^1_{\rm b} = \epsilon^2_{\rm b} \equiv \epsilon^{\rm b}_{\perp}$ and the third is set different, to $\epsilon^3_{\rm b} = \epsilon^{\rm b}_{\parallel}$. A stronger (i.e. more negative) $\epsilon^{\rm b}_{\perp}$ favors intra-ring binding whereas $\epsilon^{\rm b}_{\parallel}$ is responsible for inter-ring binding.

In addition to the above terms, each subunit has at its center of mass a spherical excluder of radius $0.2l_0$ to prevent subunit overlaps. Finally, to prevent extreme distortions of subunits, maximum edge length fluctuations are limited to $l_0/2 < l < 3l_0/2$.

### 2. *Coarse-graining*

Our model is motivated by the triangular DNA origami subunits developed in Sigl et al.[2], in which subunits bind through lock-and-key 'patches' along subunit edges in which attractive interactions are generated through blunt-end

stacking of unsatisfied nucleotides. Therefore, in our model we define attractive bonds along subunit edges (rather than at vertices as in the RG model). In particular, attractive bonds occur at each shared pair of subunit edges with the same type. Because the interactions in the experimental system are driven by nucleotide stacking, they are extremely short-ranged in comparison to the subunit size (the subunit edge lengths are approximately 60 nm). Therefore, in our simulations we avoid resolving the short length scale fluctuations in separation distance between bound edges and their associated vertices by coarse-graining as follows.

A microstate $i$ is defined as the position of all the $3n_\mathrm{s}$ vertices of $n_\mathrm{s}$ subunits: $i \rightarrow (\vec{x}_1, \vec{x}_2, ...\vec{x}_{3n_\mathrm{s}})$ The grand canonical probability *density* of finding the system around state $i$ is

$$f(i) = \frac{P(\vec{x}_1, \vec{x}_1 + d\vec{x}_1; ...; \vec{x}_1, \vec{x}_{n_s} + d\vec{x}_{n_s})}{d\vec{x}_1 d\vec{x}_2 ... d\vec{x}_{3n_\mathrm{s}}} = \frac{1}{Z_\Omega} \frac{e^{\beta n_\mathrm{s} \mu}}{\lambda^{9n_\mathrm{s}}} e^{-\beta E_i} \tag{5}$$

where $\mu$ is the chemical potential and $\lambda^3$ is the standard state volume. This probability density has the dimensions of 1/volume$^{3n_\mathrm{s}}$ corresponding to all the $3n_\mathrm{s}$ vertices of the subunits. Due to bonds, however, some pairs of vertices are confined within a *binding volume* $v_\mathrm{a}$. We consider a square-well potential so that the binding energy is constant within this volume. Analogous to Ref. [1], we can then coarse-grain to avoid resolving intra-bond fluctuations. We assume that fluctuations of bound edges are sufficiently small that each pair of vertices at either end of a bound edge pair are constrained within a *binding volume* $v_\mathrm{a}$. Note that we constrain vertices rather than edges so that the coarse-grained microstate can be represented in terms of positions of vertices rather than edges, which is easier to implement computationally. In the coarse-grained system, a coarse microstate is specified by the coordinates corresponding to the independent vertex degrees of freedom (with 1 degree of freedom for each bound vertex group and unbound vertex): $\Gamma \rightarrow (\vec{x}_1, \vec{x}_2, ...\vec{x}_{n_\mathrm{v}})$, where $n_\mathrm{v}$ is the number of independent bound vertex groups and free vertices. The probability of such a coarse-grained state is given by the net weight of all the corresponding fine-grained microstates:

$$\rho(\Gamma) = \int_{\{v_\mathrm{a}\}} f(i) \mathrm{d}^{\mathrm{n_{VB}}} \vec{x} \tag{6}$$

where $n_\mathrm{VB}$ is the number of vertex-bonds and is given by $n_\mathrm{VB} = 3n_\mathrm{s} - n_\mathrm{v}$. For simplicity, we take the limit in which $\sqrt[3]{v_\mathrm{a}}$ is small in comparison to the length scale over which the elastic energy varies, so that the energy is constant within the bound volume $v_\mathrm{a}$. Then $f(i)$ is a constant, and the probability density is given by

$$\rho(\Gamma) = \frac{1}{Z_\Omega} v_\mathrm{a}^{n_\mathrm{VB}} \frac{e^{\beta n_\mathrm{s} \mu}}{\lambda^{9n_\mathrm{s}}} e^{-\beta E_\Gamma} \tag{7}$$

where $E_\Gamma$ is the total energy of state $\Gamma$ (including stretching, bending and binding energies). The coarse graining process is illustrated in Fig. 1.

*Differences from the RG model [1].* First, in our model attractive bonds are defined along shared edges, while attractive bonds are counted at grouped vertices in the RG model. Thus, in our model the number of bonds $n_\mathrm{b}$ for a given configuration is equal to the number of shared edges, whereas in the RG model it would be equal to the number vertex bonds, $n_\mathrm{VB}$. However, the Hamiltonian for the elastic energy of the triangulated sheet and the corresponding Monte Carlo algorithm are much more straightforward to define in terms of a set of vertex positions rather than edge positions and orientations. Therefore, in our simulations we track vertex positions, by following the coarse-graining procedure described above. The distinction between attractions at edge- or vertex-pairs does not lead to qualitative differences between our model in the RG model, but it does imply that the binding affinity values $\epsilon_\mathrm{b}$ and the binding volume $v_\mathrm{a}$ must be treated as independent parameters in our model, since in general the number of bound vertices is not identical to the number of bound edges. Note that both definitions (bonds along edges or bonds at vertex pairs) involve approximations to the rotational and translational entropy penalties associated with subunit binding, since they assume a constant entropy penalty for each vertex degree of freedom that is lost within a bound vertex group, independent of the local environment (i.e., the number of bonds that a given subunit has) [3, 4].

Second, because we are modeling independent triangular subunits binding along edges, each unbound edge in the graph (those edges at the boundary of the structure) correspond to a single physical subunit edge, while bound edges (those in the structure interior) each correspond to two physical subunit edges. Therefore, in our model we set the stretching modulus for a bound edge to be twice that of a free edge. In the RG model all edges have the same stretching modulus.

### 3. *Implementation and data structure*

The simulation is implemented on top of the OpenMesh library [5]. Subunits are implemented as triangular mesh elements. OpenMesh uses the halfedge data structure which is suitable to implement triangles with directed normals

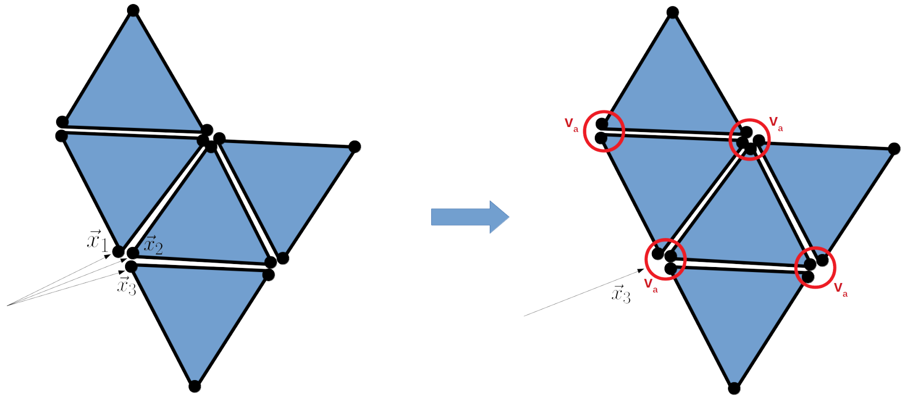


FIG. 1. Coarse-graining of an example cluster configuration. In this configuration, the number of subunits is $n_{\rm s} = 5$, the number of initial (before coarse-graining) vertices is $3n_{\rm s} = 15$, and the number of vertices after coarse-graining is $n_{\rm v} = 7$. The red circles indicate bound vertex groups, and the number of vertex degrees of freedom that have been eliminated by coarse-graining in this configuration is $n_{\rm VB} = 1 + 3 + 2 + 2 = 8 = 3n_{\rm s} - n_{\rm v}$. Motivated by DNA origami subunits in Sigl et al. [2], the attractive interactions (i.e. 'bonds') in this model occur along edge-pairs of the same type shared by two subunits. In this configuration there are $n_{\rm b} = 4$ bonds.

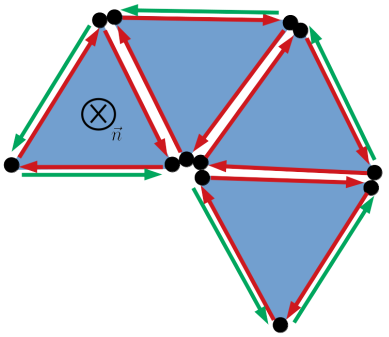


FIG. 2. The halfedge data structure used by OpenMesh. Each edge is represented by two directed edges. Boundary edges are no exception and thus are represented by a non-boundary halfedge and a boundary halfedge (in green). This latter is irrelevant for our model. Directed edges allow for the unambiguous definition of face normals, for efficient iterations of the element's neighborhood as well as boundary iterations.

(Fig 2). The directed halfedges allow for a clockwise iteration through the boundary of a triangle, which makes the two faces of the triangles distinguishable. Only halfedges with opposite orientations can bind together, making it impossible to form a Mobius strip, for example. The data structure and the resulting iterators in OpenMesh allow for an easy and efficient iteration over the neighborhood of mesh elements (vertices, edges and faces). The implementation of mesh element rearrangements is less straightforward, but we implemented it via the insertion and removal of virtual triangles. In addition, OpenMesh allows for the storage of various properties on mesh elements, allowing storage of edge types and face types stored on the elements. To improve readability in the upcoming sections, we will not represent halfedges separately.

## II. THE MONTE CARLO MOVES

In this section we detail the Monte Carlo moves of the simulation. Our algorithm has 11 moves: vertex displacement, simple subunit insertion/deletion, wedge insertion/deletion, wedge fusion/fission, crack fusion/fission, and edge fusion/fission.

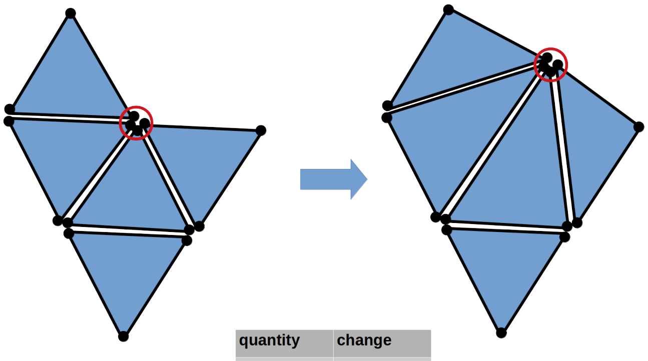

| quantity | change |
|---|---|
| $n_s$ | 0 |
| $n_{VB}$ | 0 |
| $n_b$ | 0 |

FIG. 3. Vertex move. A vertex is randomly displaced and the move is accepted according to the usual Metropolis probability.

*Detailed balance.* For the transition between state $\Gamma$ and $\Gamma'$ detailed balance corresponds to [1, 6]:

$$P(\Gamma) \times \alpha(\Gamma \to \Gamma') \times p_{\mathrm{acc}}(\Gamma \to \Gamma') = P(\Gamma') \times \alpha(\Gamma' \to \Gamma) \times p_{\mathrm{acc}}(\Gamma' \to \Gamma) \tag{8}$$

where $\alpha(\Gamma \to \Gamma')$ is the probability of generating a $\Gamma \to \Gamma'$ move attempt (trial), $p_{\mathrm{acc}}(\Gamma \to \Gamma')$ is the probability of accepting the move, and $P(\Gamma) = \rho(\Gamma)\mathrm{d}^{\mathrm{n_v}(\Gamma)}\vec{x}$ is the equilibrium probability of finding a system in a voxel of volume $\mathrm{d}^{\mathrm{n_v}(\Gamma)}\vec{x}$.

Next, we use Eq. (8) to define the acceptance criteria for each MC move. The acceptance criteria are derived in detail for the wedge fusion/fission move; the steps to follow are the same for all other moves.

## A. Vertex displacement

In this move, a vertex is randomly selected, a random uniform displacement is drawn, and the vertex is displaced to its new position according to:

$$x \to x + \mathcal{U}(-d_{\mathrm{max}}, d_{\mathrm{max}}) \tag{9}$$
$$y \to y + \mathcal{U}(-d_{\mathrm{max}}, d_{\mathrm{max}}) \tag{10}$$
$$z \to z + \mathcal{U}(-d_{\mathrm{max}}, d_{\mathrm{max}}) \tag{11}$$

with $d_{\mathrm{max}}$ the maximum displacement. The move is accepted with a probability $p_{\mathrm{acc}} = \exp(-\Delta E/k_{\mathrm{B}}T)$ where $\Delta E$ is the (bending plus stretching) energy change due to the displacement. The parameter $d_{\mathrm{max}}$ can be adjusted during a burn-in period to optimize convergence to equilibrium. Generally optimal values are on the order of the typical length scale of thermal fluctuations dictated by the elastic energy, leading to acceptance probabilities on the order of 50%. In our simulations typical values are between $d_{\mathrm{max}} = [0.01l_0, 0.1l_0]$. The vertex displacement move is illustrated in Fig 3: the number of subunits $n_{\mathrm{s}}$, number of vertices $n_{\mathrm{v}}$, number of vertex bonds $n_{\mathrm{VB}}$ and number of bonds $n_{\mathrm{b}}$ remains unchanged during this move.

## B. Simple insertion / removal

### 1. *Simple insertion*

In this move, an edge is randomly selected from the set of all boundary edges, where a new subunit will be attached. The number of such boundary edges is $n_{\mathrm{e}}$. Subunits can be inserted in $n_{\mathrm{r}}$ different rotations, where $n_{\mathrm{r}}$ is the number of distinct rotational states for a subunit which has one edge aligned with the edge of a neighboring subunit. For our triangular subunits with three distinct edge types, $n_{\mathrm{r}} = 3$. In our algorithm, during insertion of a subunit its rotational state is chosen randomly from the set of three possibilities. If the aligned edge is not complementary to

the type of the boundary edge, then the move is rejected. In this work, the two edges must be of the same type to be complementary.

The positions of two of the new subunit's vertices (those at either end of the edge being bound) are set equal to the positions of the corresponding vertices of the boundary edge to which it is binding. The third vertex position is randomly chosen from within a volume $v_{\rm add}$ centered at the equilibrium position of the new vertex.

Thus, the attempt probability for a simple insertion is given by:

$$\alpha(i \to j) = n_{\rm e} k_{\rm i} \tau n_{\rm r} \times \frac{1}{n_{\rm e} n_{\rm r} (v_{\rm add}/{\rm d}\vec{x})}. \tag{12}$$

Then, applying Eq. (8) and the attempt probability for the reverse move (simple deletion, presented next, Eq. (14)), the acceptance probabilities for a simple insertion is

$$p_{\rm acc}(i \to j) = \min \left[ 1, \frac{v_{\rm a}^2 v_{\rm add}}{\lambda^9} \exp[-(\Delta E_{i \to j} - \mu)/k_{\rm B}T] \right]. \tag{13}$$

$\Delta E_{i \to j}$ is the energy change due to the move and includes the stretching energy of the newly inserted subunit, its bending energy along the shared edge, and the binding energy due to the creation of an extra bond. During this move, one new (edge) bond and two new vertex bonds are created; i.e. $n_{\rm b} \to n_{\rm b} + 1$ and $n_{\rm VB} \to n_{\rm VB} + 2$. Moreover, the number of vertices in the structure increases by one, $n_{\rm v} \to n_{\rm v} + 1$.

#### 2. *Simple removal*

The reverse move to simple insertion is simple removal. Subunits that can be deleted with this move are those with two boundary edges. The number of simply removable subunits is $n_{\rm sr}$. One of these is selected randomly, so the attempt probability is

$$\alpha(j \to i) = n_{\rm sr} k_{\rm i} \tau \times \frac{1}{n_{\rm sr}} \tag{14}$$

and, using Eq. (8) and Eq. (12), the acceptance probability is

$$p_{\rm acc}(j \to i) = \min \left[ 1, \frac{\lambda^9}{v_{\rm a}^2 v_{\rm add}} \exp[-(\Delta E_{j \to i} + \mu)/k_{\rm B}T] \right] \tag{15}$$

During this move, the structure loses one (edge) bond and two vertex bonds; $n_{\rm b} \to n_{\rm b} - 1$ and $n_{\rm VB} \to n_{\rm VB} - 2$. The number of vertices in the structure decreases by one, $n_{\rm v} \to n_{\rm v} - 1$.

If there are multiple species with chemical potentials $\mu_k$, detailed balance must be satisfied for each species, individually. Moreover, each species can have different insertion rates $k_{\rm i}^k$.

To keep $\alpha < 1$, we ensure that the insertion rate $k_{\rm i}$ constrained by

$$n_{\rm e} k_{\rm i} \tau n_{\rm r} < 1 \tag{16}$$

$$n_{\rm sr} k_{\rm i} \tau < 1 \tag{17}$$

In equilibrium, one can use adaptive rates, i.e. reduce $k_i$ on the run if the above condition is not satisfied. In that case, sampling is not taken for the ensuing several time steps. Alternatively, the rates may be set to a low enough value from the beginning and only tested on the run to ensure that the $\alpha < 1$ condition is satisfied. This latter technique is appropriate for dynamical runs as it keeps the rates constant throughout the simulation.

Moreover, we must ensure that $v_{\rm add}$ is large enough so that the vertex does not leave the $v_{\rm add}$ volume during structural relaxation moves; otherwise the insertion/deletion moves would not be reversible and the detailed balance would be violated. For a better convergence, one could choose a gaussian distribution $\mathcal{N}(\vec{r})$ for the position of the new vertex instead of a uniform distribution $1/v_{\rm add}$. In this case, this distribution has to be accounted for in the acceptance probabilities $p_{\rm acc}(i \to j)$ and $p_{\rm acc}(j \to i)$.

### C. Wedge insertion/removal

#### 1. *Wedge insertion*

Wedges are positions in the structure where a triangle can be inserted via attaching to two edges (Fig. 5). In a wedge move, we pick randomly from the set of available wedge positions in the structure, and pick a random orientation for

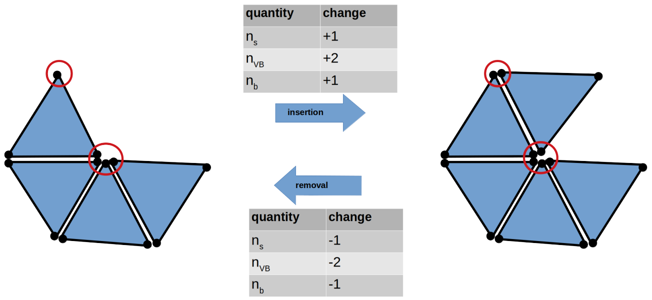


FIG. 4. Simple insertion and removal.

the new subunit. Denoting the number of wedge positions in a given structure as $n_{\rm w}$, the attempt probability for a wedge move is

$$\alpha(i \to j) = n_{\rm w} k_{\rm i} \tau n_{\rm r} \times \frac{1}{n_{\rm r} n_{\rm w}} \tag{18}$$

In contrast to the simple insertion move, there is no need for random vertex displacement in a wedge move because all three vertices of the new subunit are fixed by the three vertices of the wedge position. Combining Eq. (18) and the attempt probability for wedge removal (Eq. (20)), The acceptance probability for a wedge insertion is

$$p_{\rm acc}(i \to j) = \min\left[1, \frac{v_{\rm a}^3}{\lambda^9} \exp[-(\Delta E_{i\to j} - \mu)/k_{\rm B}T]\right]. \tag{19}$$

During a wedge insertion, two edge bonds and three vertex bonds are created; i.e., $n_{\rm b} \to n_{\rm b} + 2$ and $n_{\rm VB} \to n_{\rm VB} + 3$, but the number of vertices is unchanged, $n_{\rm v} \to n_{\rm v}$. $\Delta E_{i\to j}$ includes the binding energy of the two newly formed bonds, the two bending energies along the two newly bound edges and the stretching energy of the newly inserted subunit.

### *2. Wedge removal*

The reverse move of wedge insertion is wedge removal. In a wedge removal, we randomly choose one of the removable wedges from a given structure. With the number of removable wedges as $n_{\rm wr}$, the attempt probability is

$$\alpha(j \to i) = n_{\rm wr} k_{\rm i} \tau \times \frac{1}{n_{\rm wr}}. \tag{20}$$

Using Eq. (18), the acceptance probability for a wedge removal is then

$$p_{\rm acc}(j \to i) = \min\left[1, \frac{\lambda^9}{v_{\rm a}^3} \exp[-(\Delta E_{j\to i} + \mu)/k_{\rm B}T]\right]. \tag{21}$$

We have the following constraints on rates $k_{\rm i}$ for wedge insertion/removal:

$$n_{\rm w} k_{\rm i} \tau n_{\rm r} < 1 \tag{22}$$

$$n_{\rm wr} k_{\rm i} \tau < 1 \tag{23}$$

As for simple insertion and removal, in the case of multiple species, detailed balance is satisfied for each species separately for wedge insertion/removal.

## D. Wedge fusion / fission

### *1. Wedge fusion*

In this move, a *fusable wedge* is closed, without inserting a new subunit (Fig 6). That is, the two vertices on either side of the wedge opening are merged into a single vertex. Fusable wedges are vertex pairs that i) form a wedge (as in the case of wedge insertion) and ii) are within a separation distance of $l_{\rm fuse}$.

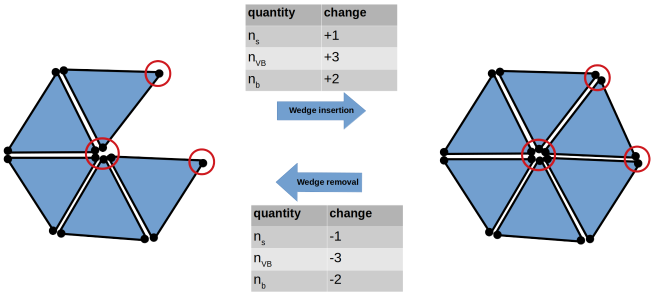


FIG. 5. Wedge insertion and removal.

Denoting the number of fusible wedge positions as $n_{\mathrm{w}}$, in each MC step, a wedge fusion is attempted with probability $n_{\mathrm{w}} k_{\mathrm{wf}} \tau$, where $k_{\mathrm{wf}}$ is an adjustable parameter controlling the relative probability of attempting wedge fusion. Then, a wedge position is selected randomly from the set of all $n_{\mathrm{w}}$ fusible wedges. The attempt probability is thus

$$\alpha(i \to j) = n_{\mathrm{w}} k_{\mathrm{wf}} \tau \times \frac{1}{n_{\mathrm{w}}}. \tag{24}$$

Using Eqs. (24) and (26), the acceptance probability for fusion moves is

$$p_{\mathrm{acc}}(i \to j) = \min\left[1, \frac{v_{\mathrm{a}}}{v_{\mathrm{fuse}}} \exp(-\Delta E_{i\to j}/k_{\mathrm{B}}T)\right] \tag{25}$$

where $v_{\mathrm{fuse}} = (4\pi/3)(l_{\mathrm{fuse}}/2)^3$ is the volume of a sphere with diameter $l_{\mathrm{fuse}}$, and $\Delta E_{i\to j}$ is the energy change due to the fusion, including changes in bending, stretching, and binding energies. A fusion move increases the number of edge bonds and vertex bonds by one, $n_{\mathrm{b}} \to n_{\mathrm{b}} + 1$ and $n_{\mathrm{VB}} \to n_{\mathrm{VB}} + 1$; the factor of $v_{\mathrm{a}}$ appears in Eq. (25) to account for the latter.

### 2. *Wedge fission*

Wedge fission, in which a wedge is opened, is the reverse of the wedge fusion move. Fissionable edges are those edges that can be split along their boundary vertex to obtain a wedge. Denoting the number of such edges as $n_{\mathrm{f}}$, the probability of attempting a wedge fission move during an MC step is $n_{\mathrm{f}} k_{\mathrm{wf}} \tau$. If a fission move is attempted, then an edge is selected randomly from the $n_{\mathrm{f}}$ fissionable edges. The position of one of the new vertices is selected randomly within the sphere of volume $v_{\mathrm{fuse}}$ centered at the original position of the merged vertices, and the other new vertex is placed in the opposite direction from the original position, at the same distance. Thus, the attempt generation probability is

$$\alpha(j \to i) = n_{\mathrm{f}} k_{\mathrm{wf}} \tau \times \frac{1}{n_{\mathrm{f}}(v_{\mathrm{fuse}}/\mathrm{d}\vec{x})} \tag{26}$$

and the acceptance probability is

$$p_{\mathrm{acc}}(j \to i) = \min\left[1, \frac{v_{\mathrm{fuse}}}{v_{\mathrm{a}}} \exp(-\Delta E_{j\to i}/k_{\mathrm{B}}T)\right] \tag{27}$$

We verify that detailed balance holds between wedge fusion and fission as follows. There are two cases to consider:

1. $(v_{\mathrm{fuse}}/v_{\mathrm{a}}) \exp(-\Delta E_{j\to i}/k_{\mathrm{B}}T) < 1 \Leftrightarrow (v_{\mathrm{a}}/v_{\mathrm{fuse}}) \exp(-\Delta E_{i\to j}/k_{\mathrm{B}}T) > 1$

   In this case, $p_{\mathrm{acc}}(i \to j) = 1$ and $p_{\mathrm{acc}}(j \to i) = (v_{\mathrm{fuse}}/v_{\mathrm{a}}) \exp(-\Delta E_{j\to i}/k_{\mathrm{B}}T)$. Then

$$P_i \times \alpha(i \to j) \times p_{\mathrm{acc}}(i \to j) = \frac{1}{Z_\Omega} v_{\mathrm{a}}^{n_{VB,i}} \exp[-(E_i - \mu n_{s,i})/k_{\mathrm{B}}T] \frac{1}{\lambda^{9 n_{s,i}}} \times \mathrm{d}^{\mathrm{n_{v,i}}}\vec{x} \times k_{wf}\tau \tag{28}$$

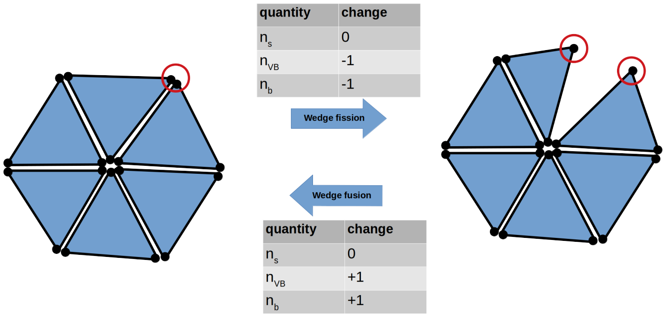


FIG. 6. Wedge fusion and fission.

and

$$P_j \times \alpha(j \to i) \times p_{\rm acc}(j \to i) = \frac{1}{Z_\Omega} v_{\rm a}^{n_{VB,j}} \exp[-(E_j - \mu n_{s,j})/k_{\rm B}T] \frac{1}{\lambda^{9n_{s,j}}} \times {\rm d}^{\rm n_{v,j}}\vec{x} \tag{29}$$

$$\times\, k_{wf}\tau {\rm d}\vec{x}/v_{\rm fuse} \times (v_{\rm fuse}/v_{\rm a}) \exp(-\Delta E_{j\to i}/k_{\rm B}T) \tag{30}$$

Using: $\Delta E_{j\to i} = E_i - E_j$, $n_{s,i} = n_{s,j}$ (because the move leaves the subunit number unchanged), $n_{VB,i} = n_{VB,j} - 1$ (one vertex bond is broken upon fission) and $n_{v,i} = n_{v,j} + 1$ (an extra vertex is being born upon fission), we see that the two are equal and detailed balance holds.

2. $(v_{\rm fuse}/v_{\rm a}) \exp(-\Delta E_{j\to i}/k_{\rm B}T) > 1 \Leftrightarrow (v_{\rm a}/v_{\rm fuse}) \exp(-\Delta E_{i\to j}/k_{\rm B}T) < 1$

   In this case, $p_{\rm acc}(i \to j) = (v_{\rm a}/v_{\rm fuse}) \exp(-\Delta E_{i\to j}/k_{\rm B}T)$ and $p_{\rm acc}(j \to i) = 1$. Then

$$P_i \times \alpha(i \to j) \times p_{\rm acc}(i \to j) = \frac{1}{Z_\Omega} v_a^{n_{VB,i}} \exp[-(E_i - \mu n_{s,i})/k_{\rm B}T] \frac{1}{\lambda^{9n_{s,i}}} \times {\rm d}^{\rm n_{v,i}}\vec{x} \times k_{wf}\tau \tag{31}$$

$$\times\, (v_{\rm a}/v_{\rm fuse}) \exp(-\Delta E_{i\to j}/k_{\rm B}T) \tag{32}$$

and

$$P_j \times \alpha(j \to i) \times p_{\rm acc}(j \to i) = \frac{1}{Z_\Omega} v_a^{n_{VB,j}} \exp[-(E_j - \mu n_{s,j})/k_{\rm B}T] \frac{1}{\lambda^{9n_{s,j}}} \times {\rm d}^{\rm n_{v,j}}\vec{x} \tag{33}$$

$$\times\, k_{wf}\tau {\rm d}\vec{x}/v_{\rm fuse} \tag{34}$$

Using again $\Delta E_{j\to i} = E_i - E_j$, $n_{s,i} = n_{s,j}$, $n_{VB,i} = n_{VB,j} - 1$ and $n_{v,i} = n_{v,j} + 1$, detailed balance holds.

Note that detailed balance is satisfied regardless of the values of $k_{\rm wf}\tau$ or $v_{\rm fuse}$, but as with all of the move frequencies these parameters can be optimized during burn-in to accelerate convergence to the equilibrium distribution $P(i)$. In our simulations, we find that the optimal value of $v_{\rm fuse}$ is on the order of the optimal value of $d_{\rm max}$ for analogous reasons: if $v_{\rm fuse}$ is too small there will be very few vertex pairs identified as fusable, so $n_{\rm w}$ will be low. If $v_{\rm fuse}$ is too large, there will be many fusion candidates but most fusion attempts will be rejected due to the large elastic energy change necessary for the merging deformation.

Most importantly, we note the constraint on the parameters $k_{\rm wf}\tau$ to ensure that generation probabilities do not become larger than unity. Because each attempt is generated as a three step process, using three probabilities, one has to ensure that all those probabilities are less than 1. Specifically,

$$n_{\rm w} k_{\rm wf}\tau < 1 \tag{35}$$

$$n_{\rm f} k_{\rm wf}\tau < 1. \tag{36}$$

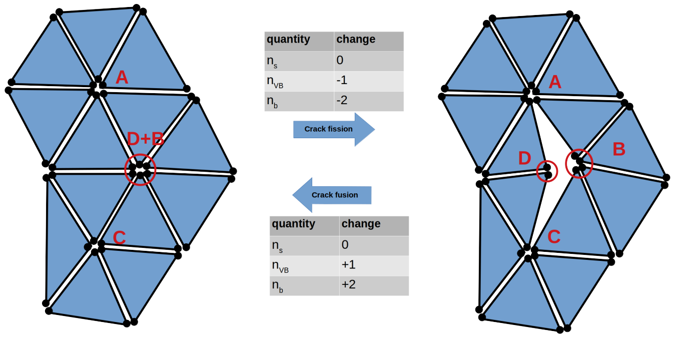


FIG. 7. Crack fusion and fission.

## E. Crack fusion / fission

### 1. *Crack fusion*

Crack fusion closes a crack within the structure; i.e., two adjacent pairs of edges are merged (Fig. 7). Cracks are identified as 4-edge-length holes inside the structure. If the vertices of the hole are labeled A, B, C, D then the polygon ABCD forms a closed loop (see Fig. 7). The crack can be closed by either merging vertices A and C (and correspondingly edges CD to DA and AB to BC) or by merging vertices B and D (and correspondingly edges AD to AB and CD to CB). Each 4-edge-length loop thus defines two potential fusable cracks. However, an additional condition for a crack to be fusable is that its merging vertices must be within a distance $l_{\mathrm{fuse}}$ (A and C or D and B in this example). In this work, we have set the crack fusion volume to be the same as that for wedge fusion to reduce the number of parameters, but it is not necessary that they be the same.and the acceptance probability is

$$p_{\mathrm{acc}}(i \to j) = \min\left[1, \frac{v_{\mathrm{a}}}{v_{\mathrm{fuse}}} \exp(-\Delta E_{i\to j}/k_{\mathrm{B}}T)\right] \tag{37}$$

There are two edge bonds and one vertex bond formed during a crack fusion.

### 2. *Crack fission*

The reverse move for crack fusion is crack fission. With the number of potential cracks as $n_{\mathrm{cf}}$:

$$\alpha(j \to i) = n_{\mathrm{cf}} k_{\mathrm{cf}} \tau \times \frac{1}{n_{\mathrm{cf}}(v_{\mathrm{fuse}}/\mathrm{d}\vec{x})} \tag{38}$$

$$p_{\mathrm{acc}}(j \to i) = \min\left[1, \frac{v_{\mathrm{fuse}}}{v_{\mathrm{a}}} \exp(-\Delta E_{j\to i}/k_{\mathrm{B}}T)\right] \tag{39}$$

As for the case of wedge fusion/fission, the crack fusion attempt frequency parameter $k_{\mathrm{cf}}$ is constrained by the conditions maintaining probabilities smaller than unity:

$$n_{\mathrm{c}} k_{\mathrm{cf}} \tau < 1 \tag{40}$$

$$n_{\mathrm{cf}} k_{\mathrm{cf}} \tau < 1 \tag{41}$$

$$\tag{42}$$

## F. Edge fusion / fission

### 1. *Edge fusion*

During this move two non-neighbor edges are fused (Fig. 8). Fusable edges are non-neighboring edge pairs whose corresponding vertices are within a separation distance $l_{\mathrm{fuse}}$. Since edges are directed, they can only fuse such that,

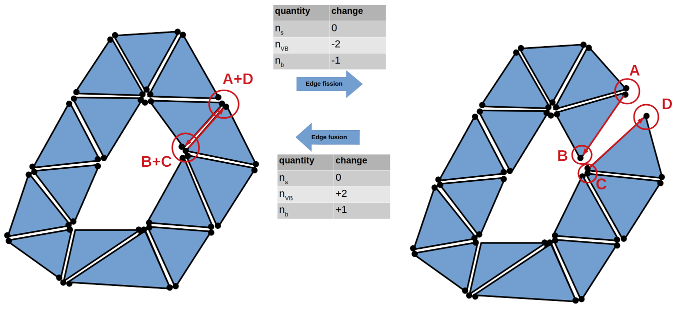


FIG. 8. Edge fusion and fission.

after fusion, they point in the opposite direction. Assuming the edges to be fused are $A \to B$ and $C \to D$ (see Fig. 8), vertex $A$ will merge into vertex $D$ and vertex $B$ will merge into vertex $C$. Edges are counted as fusable if $A$ is within a distance $l_{\rm fuse}$ to $D$ and $B$ is also within a distance $l_{\rm fuse}$ to $C$. The attempt probability is analogous to that for wedge and crack fusion/fission,

$$\alpha(i \to j) = n_{\rm e} k_{\rm ef} \tau \times \frac{1}{n_{\rm e}} \tag{43}$$

with $n_{\rm e}$ the number of fusable edges and $k_{\rm ef}$ the edge fusion frequency parameter. The acceptance probability is

$$p_{\rm acc}(i \to j) = \min\left[1, \left(\frac{v_{\rm a}}{v_{\rm fuse}}\right)^2 \exp(-\Delta E_{i\to j}/k_{\rm B}T)\right] \tag{44}$$

During edge fusion, one edge bond and two vertex bonds are created.

### 2. *Edge fission*

Edge fission is the reverse move of edge fusion. $n_{\rm ef}$ is the number of breakable edges, that is, those edges that have both vertices on the boundary and which would not result in breaking the structure apart.

$$\alpha(j \to i) = n_{\rm ef} k_{\rm ef} \tau \times \frac{1}{n_{\rm ef}(v_{\rm fuse}/{\rm d}\vec{x})^2} \tag{45}$$

The factor $1/(v_{\rm fuse})^2$ arises because we must select a random position for each pair of vertices, independently. The acceptance probability is then

$$p_{\rm acc}(j \to i) = \min\left[1, \left(\frac{v_{\rm fuse}}{v_{\rm a}}\right)^2 \exp(-\Delta E_{j\to i}/k_{\rm B}T)\right]. \tag{46}$$

To maintain probabilities within unity, the edge fusion frequency parameter $k_{\rm ef}$ is constrained by

$$n_{\rm e} k_{\rm ef} \tau < 1 \tag{47}$$
$$n_{\rm ef} k_{\rm ef} \tau < 1. \tag{48}$$

## III. UMBRELLA SAMPLING, PARALLEL TEMPERING, AND FREE ENERGY CALCULATIONS

### 1. *Bias potentials.*

The grand potential (up to an $n$-independent constant $k_{\rm B}T \ln Z_\Omega$), $\Omega_n$, can be computed as $\Omega_n = -k_{\rm B}T \ln P(n)$ where $P(n)$ is the equilibrium probability of observing $n$ subunits in the structure. While $P(n)$ can in principle be computed by tabulating a histogram of cluster sizes during an unbiased simulation, in practice only the high-probability

cluster sizes will result in statistically significant sampling. To improve sampling, we perform umbrella sampling, with independent windows in which a harmonic bias potential $U_\mathrm{b} = k_\mathrm{umbrella}(n - n_0)^2/2$ that restrains the cluster size to remain near $n_0$, with $k_\mathrm{umbrella}$ the strength of the bias potential, and each window can have different values of $n_0$ and $k_\mathrm{umbrella}$. We perform simulations in which histograms corresponding to the biased probability distribution $P_\mathrm{bias}(n)$ are measured; the biased histograms are then combined and unbiased using the Weighted Histogram Analysis Method [7] to obtain $\Omega_n$. We used the Bayes-WHAM implementation by Ferguson [8].

The interaction free energy $F_n$ is then given by $F_n = \Omega_n + \mu n$, with $\mu$ the chemical potential. Importantly, measurements performed at different chemical potentials $\mu$ should result in the same $F_n$, since $F_n$ represents the cluster interaction free energy which is independent of the bath concentration. However, different imposed values of $\mu$ will 'tilt' the free energy landscape and thus favor sampling different values of $n$ for a given bias potential. Therefore, it is useful to combine the imposed chemical potential into the bias potential as:

$$U_\mathrm{b}(n, n_0) = k_\mathrm{umbrella}\frac{(n - n_0)^2}{2} - \mu(n - n_0) \tag{49}$$

The $n_0$ in the linear term does not affect the computed value of $F_n$ (which depends only on $\partial U_\mathrm{b}/\partial n$) but is convenient for numerical reasons in solution of the WHAM equations. The simulation is then performed with a Hamiltonian $H(\Gamma) = E(\Gamma) + U_\mathrm{b}(n, n_0)$.

### 2. *Parallel tempering*

Convergence of umbrella sampling calculations is poor when there are slow degrees of freedom in addition to reaction coordinate being biased (which is the cluster size $n$ in our case). Moreover, because our reaction coordinate is discrete, sampling may be poor in cases where the underlying free energy landscape has a jump which is large in comparison to $k_\mathrm{B}T$ over a single subunit. Therefore, to improve sampling, we performed parallel tempering between different umbrella sampling windows and replicas at different temperatures. In particular, we simultaneously performed simulations with 3 different temperatures, 4 umbrella spring constants $k_\mathrm{umbrella}$ and 3 chemical potentials $\mu$ (36 replicas in total). Swaps between these replicas were attempted randomly, with the Metropolis acceptance criteria to ensure detailed balance ([6]). In principle, results from all of these windows could be combined within WHAM, but in practice combining different temperatures is impractical for a histogram-based method such as WHAM and instead requires use of 'binless' WHAM (e.g. [9, 10]). Therefore, we separately used WHAM to compute free energy profiles at each of the three temperatures. For the results in the main text, each free energy curve (and corresponding minimum point) result from exchanging between 36 replicas with $k_\mathrm{B}T = \{1, 1.1, 1.25\}$, $\mu = \{-6.5, -5.5, -5\}$, $k_\mathrm{umbrella} = \{1, 1.5, 2, 2.5\}$. Technically, a non-unit temperature is equivalent to rescaling the elastic moduli, binding energies, chemical potential and the umbrella spring constant by the same factor, however, it is easier to implement with having the temperature as a separate parameter.

## IV. MAPPING TO TARGET CURVATURES FROM LOCAL DIHEDRALS

Here we briefly outline the mapping between preferred dihedrals between adjacent triangular edges and the *target* values for target (triangulated) surface. Notably, the target shape prefers a non-zero Gaussian curvature that is incompatible with the equilateral edge lengths, and hence, we deduce the values of the target curvature from *unfrustrated strips* along nearest neighbor rows of triangles. Consider for example, a row shown in Fig. 9(a) corresponding to an alternating sequence of dihedrals, $\theta_i$ and $\theta_j$. The curvature along this row is defined by considered the circle defined by three consecutive vertices along the row, see the green, blue and yellow points in Fig. 9(a) . These points define a vector $\mathbf{R}(\theta_i, \theta_j)$ that points from the central vertex to the center of curvature, such that the local radius of curvature is its length. As the local discrete approximation to the curvature of these edges is $\mathbf{R}(\theta_i, \theta_j)/|\mathbf{R}(\theta_i, \theta_j)|^2$, the discrete approximation of the *normal curvature* of a surface spanned by the triangular faces is given by,

$$\kappa(\theta_i, \theta_j) = \frac{\mathbf{n} \cdot \mathbf{R}(\theta_i, \theta_j)}{|\mathbf{R}(\theta_i, \theta_j)|^2} = \frac{2\sqrt{3}(\sin\theta_i + \sin\theta_j)\big(\cos\theta_i + \cos\theta_j + \cos\theta_i\cos\theta_j - 2\sin\theta_i\sin\theta_j - 3\big)}{\ell_0\big[4\cos\theta_i + 4\cos\theta_j - 8\cos(\theta_i - \theta_j) + 3\cos(2\theta_i) + 3\cos(2\theta_j) - 6\big]} \tag{50}$$

where $\mathbf{n}$ is the normal to the central triangle, and $\ell_0$ is the preferred edge length. For small angles this row curvature reduces to the simple form

$$\kappa(\theta_i \ll 1, \theta_j \ll 1) \simeq \frac{\sqrt{3}(\theta_i + \theta_j)}{2\ell_0}. \tag{51}$$

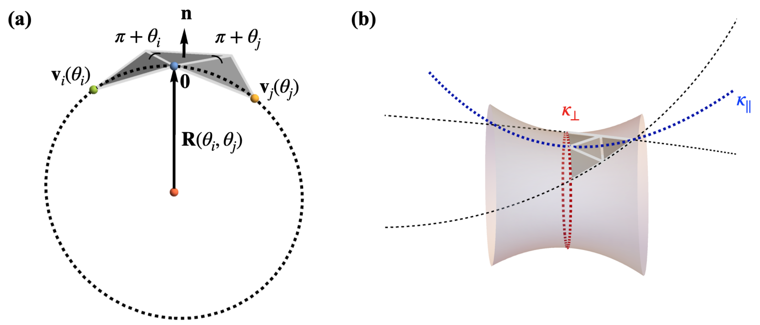


FIG. 9. Schematic for defining target curvatures from preferred dihedrals of triangular subunits. (a) shows the definition of target curvature along a row of triangles with consecutive dihedrals, $\theta_i$ and $\theta_j$, based on the circle defined by 3 consecutive vertices, shown as green, blue, and yellow points. The vectors $\mathbf{R}(\theta_i, \theta_j)$ and $\mathbf{n}$ denote the distance from the central vertex to the center of curvature and the normal to the triangular face, respectively. (b) shows a schematic relating the two target principle curvatures, $\kappa_\perp$ and $\kappa_\parallel$, to the row curvatures of the triangular mesh, one of which lies along the principle $\perp$ direction, while the other two are shown as the dashed black curves.

Based these row curvatures, we can relate them to the principle curvatures $\kappa_\parallel$ and $\kappa_\perp$ using Euler's relation,

$$\kappa(\theta_i, \theta_j) = \kappa_\parallel(\hat{\mathbf{e}}_\parallel \cdot \hat{\mathbf{e}}_{ij})^2 + \kappa_\perp(\hat{\mathbf{e}}_\perp \cdot \hat{\mathbf{e}}_{ij})^2, \tag{52}$$

where $\hat{\mathbf{e}}_\parallel$ and $\hat{\mathbf{e}}_\perp$ are the principle directions of curvature and $\hat{\mathbf{e}}_{ij}$ is the direction of the row of alternating $ij$ bonds in the tangent plane. For trumpets, the dihedrals in the hoop ($\perp$) direction are equal to a common $\theta_2$, such that

$$\kappa_\perp = \kappa(\theta_2, \theta_2), \tag{53}$$

while the directions of the $\theta_1$ and $\theta_2$ are rotated by $2\pi/3$ with respective to this principle direction giving,

$$\kappa_\parallel = \frac{4\kappa(\theta_2, \theta_1) - \kappa(\theta_2, \theta_2)}{3}. \tag{54}$$

This alignment of the target row curvatures and principle curvature directions is shown schematically in Fig. 9(b).


[1] Grant M. Rotskoff and Phillip L. Geissler. Robust nonequilibrium pathways to microcompartment assembly. *Proceedings of the National Academy of Sciences of the United States of America*, 115(25):6341–6346, 2018.

[2] Christian Sigl, Elena M. Willner, Wouter Engelen, Jessica A. Kretzmann, Ken Sachenbacher, Anna Liedl, Fenna Kolbe, Florian Wilsch, S. Ali Aghvami, Ulrike Protzer, Michael F. Hagan, Seth Fraden, and Hendrik Dietz. Programmable icosahedral shell system for virus trapping. *Nature Materials*, 2021.

[3] Michael F. Hagan, Oren M. Elrad, and Robert L. Jack. Mechanisms of kinetic trapping in self-assembly and phase transformation. *Journal of Chemical Physics*, 135(10):1–13, 2011.

[4] Michael F. Hagan and David Chandler. Dynamic pathways for viral capsid assembly. *Biophysical Journal*, 91(1):42–54, 2006.

[5] M Botsch, S Steinberg, S Bischoff, and L Kobbelt. OpenMesh – a generic and efficient polygon mesh data structure. In *OpenSG Symposium*, 2002.

[6] Daan Frenkel and Berend Smit. Understanding molecular simulation: From algorithms to applications, 1996.

[7] Shankar Kumar, Djamal Bouzida, Robert H. Swendsen, Peter A. Kollman, and John M. Rosenberg. The weighted histogram analysis method for free-energy calculations on biomolecules. *Journal of computational chemistry*, 13(8):1011–1021, 1992.

[8] Andrew L. Ferguson. BayesWHAM: A Bayesian approach for free energy estimation, reweighting, and uncertainty quantification in the weighted histogram analysis method. *Journal of Computational Chemistry*, 38(18):1583–1605, 2017.

[9] Zhiqiang Tan, Junchao Xia, Bin W. Zhang, and Ronald M. Levy. Locally weighted histogram analysis and stochastic solution for large-scale multi-state free energy estimation. *Journal of Chemical Physics*, 144(3):40–44, 2016.

[10] Zhiqiang Tan, Emilio Gallicchio, Mauro Lapelosa, Ronald M Levy, Zhiqiang Tan, Emilio Gallicchio, Mauro Lapelosa, and Ronald M Levy. Theory of binless multi-state free energy estimation with applications to protein-ligand binding Theory of binless multi-state free energy estimation with applications to protein-ligand binding. *Journal of Chemical Physics*, 0341070341:1–14, 2012.
